# Supplementary material for: RQP-SGD: Differential Private Machine Learning through Noisy SGD and Randomized Quantization
Source: arXiv:2402.06606 source file (2024-02-09)
Supplement: Supplementary file 1 [file appendix.tex]

\appendix

\section{Proof of Theorem \ref{thm:privacy_probnsgd}}\label{app:proof_privacythm}
% \Privacythm*

\begin{proof}
    The proof relies on \renyi differential privacy (RDP)~\cite{mironov2017renyi}, a variant of the classical differential privacy~\cite{dwork2006differential,dwork2014algorithmic}. 
    A randomized mechanism $\calM:\calD\mapsto\calR$ satisfies $(\epsilon, 0)$-\renyi differential privacy if for any two adjacent sets $d,d'\in\mathcal{D}$, it holds that
    $$D_{\alpha}(\text{Pr}_{\calM(d)}\|\text{Pr}_{\calM(d')})\leq\epsilon$$
    where $D_{\alpha}(\cdot\|\cdot)$ denotes the \renyi divergence at the $\alpha$-th order.
    More specifically, for two probability distributions $P_1$ and $P_2$ defined over $\calR$, the \renyi divergence of $\alpha>1$ is
    $$D_{\alpha}(P_1\|P_2)=\frac{1}{\alpha-1}\log\mbbE_{x\sim P_2}\left(\frac{P_1(x)}{P_2(x)}\right)^{\alpha}$$
    The loss function $l(f(w_t;\cdot);\cdot)$ is $\rho$-Lipschitz with respect to $w_t$, according to Lemma 14.7 in \cite{shalev2014understanding}, for any data-label pair $(x_i,y_i)\in\calS$, we have $\|\nabla l(f(w_t;x_i);y_i\|\leq \rho$. Let $f_{sgd}(w_t;B_t)$ denotes the standard SGD update using the stochastic mini-batch $B_t$, we have
    $$f_{sgd}(w_t;B_t)= w_t-\eta\cdot\frac{1}{m}\sum^m_{j=1}\nabla l(f(w_t;x_j);y_j)$$
    where $(x_j, y_j)\in B_t$. The step 4 of Algorithm \ref{alg:ProbProjNSGD} (represented by $f_v(w_t;B_t)$) is equivalant with the following equation:
    $$f_v(w_t;B_t) = f_{sgd}(w_t;B_t) + \eta\cdot\calN(0,\sigma^2\mbbI_d)$$
    This indicates that $v_{t+1}$ follows normal distribution $\calN(f_{sgd}(w_t;B_t), \eta^2\sigma^2)$.

    Let $\Phi(\cdot)$ be the cumulative density function of $\calN(0,1)$, then for any quantization level $Q_i\in\calQ_{M,b}$, we have
    $$\scriptstyle\begin{array}{rl}
    & Pr\{\text{Proj}^R_{\calQ_{M,b}}(v_{t+1})=Q_i\} \\
    = & q\cdot[\Phi(\frac{Q_+-f_v(w_t;B_t)}{\sigma_l})-\Phi(\frac{Q_--f_v(w_t;B_t)}{\sigma_l})]+\\
    & \frac{1-q}{2^b}\cdot[\Phi(\frac{Q_+-f_v(w_t;B_t)}{\sigma_l})-\Phi(\frac{Q_--f_v(w_t;B_t)}{\sigma_l})]\\
    =& \frac{2^bq-1}{2^b-1}[\Phi(\frac{Q_+-f_v(w_t;B_t)}{\sigma_l})-\Phi(\frac{Q_--f_v(w_t;B_t)}{\sigma_l})]\\
    &+\frac{1-q}{2^b-1}
    \end{array}$$
    where $Q_-= Q_{i}-\frac{M}{2^b-1}$, $Q_+= Q_{i^*}+\frac{M}{2^b-1}$, and $\sigma_l=\eta\sigma$.

    As $f_{sgd}(w_t;B_)$ is a linear combination of the stochastic gradient, for any two adjacent $B_t, B'_t\in\calS$, we have $\scriptstyle\max\|f_{sgd}(w_t;B_t)-f_{sgd}(w_t;B_t)\|\leq C$ where $C=M-\eta\rho$. 
    And the $\infty$-th order \renyi divergence of step 5 at each iteration is
    $$D_{\infty}(\text{Proj}^R_{\calQ_{M,b}}(f_v(w_t;B_t))\|\text{Proj}^R_{\calQ_{M,b}}(f_v(w_t;B'_t)) $$
    \begin{equation}\label{eq:privacy_bound}
        \begin{array}{cl}
    % &D_{\infty}(\text{Proj}^R_{\calQ_{M,b}}(f_v(w_t;B_t))\|\text{Proj}^R_{\calQ_{M,b}}(f_v(w_t;B'_t)))\\
    =&\max\{\log\frac{\frac{2^bq-1}{2^b-1}[\Phi_+(f(B_t))-\Phi_-(f(B_t))]+\frac{1-q}{2^b-1}}{\frac{2^bq-1}{2^b-1}[\Phi_+(f(B'_t))-\Phi_-(f(B'_t))]+\frac{1-q}{2^b-1}}\}\\
    \text{where }& \Phi_+(f(B_t))=\Phi(\frac{Q_+-f_v(w_t;B_t)}{\sigma_l})\\
    & \Phi_-(f(B_t))=\Phi(\frac{Q_--f_v(w_t;B_t)}{\sigma_l})\\
    & \Phi_+(f(B'_t))=\Phi(\frac{Q_+-f_v(w_t;B'_t)}{\sigma_l})\\
    & \Phi_+(f(B'_t))=\Phi(\frac{Q_--f_v(w_t;B'_t)}{\sigma_l})
    \end{array}\end{equation}
    Fixing $b$, $C$ and $M$, the bound of (\ref{eq:privacy_bound}) is dependent on $q$ and $\sigma_l$. Let $b\geq1$, the upper bound of (\ref{eq:privacy_bound}) is dependent on the value of $f_v(w_t;B_t)$, in other words, the horizontal shift of $\Phi(\cdot)$. By adjusting the value of $\Phi_+(f(B_t))-\Phi_-(f(B_t))$,
    With the knowledge of the distribution of $f_v(w_t;B_t)$ and the bound of $f_{sgd}(w_t;B_t)$, (\ref{eq:privacy_bound}) can be obtained by adjusting the value of $\Phi_+(f(B_t))-\Phi_-(f(B_t))$. The bound of (\ref{eq:privacy_bound}) is
    $$D_{\infty}(\text{Proj}^R_{\calQ_{M,b}}(f_v(w_t;B_t))\|\text{Proj}^R_{\calQ_{M,b}}(f_v(w_t;B'_t))\leq \epsilon_t $$
    % $$\text{where }\epsilon_t=\log\frac{\frac{2^bq-1}{2^b-1}[2\Phi(\frac{a_1}{\sigma_l})-1]+\frac{1-q}{2^b-1}}{\frac{2^bq-1}{2^b-1}[\Phi(\frac{a_2}{\sigma_l})-\Phi(\frac{a_3}{\sigma_l})]+\frac{1-q}{2^b-1}}$$
    where $\epsilon_t=\log\frac{\frac{2^bq-1}{2^b-1}[2\Phi(\frac{a_1}{\sigma_l})-1]+\frac{1-q}{2^b-1}}{\frac{2^bq-1}{2^b-1}[\Phi(\frac{a_2}{\sigma_l})-\Phi(\frac{a_3}{\sigma_l})]+\frac{1-q}{2^b-1}}$, $a_1=\frac{M}{2^b-1}$,$a_2=M+\frac{M}{2^b-1}+C$, $a_3=M-\frac{M}{2^b-1}+C$. This demonstrates that each iteration of RQP-SGD is $(\infty,\epsilon_t)$-RDP with respect to the stochastic mini-batch $B_t$. According to the RDP to DP conversion~\cite{mironov2017renyi}, it is equivalent with $(\epsilon_t,0)$-DP. 

    RQP-SGD performs total $T$ iterations, and at each iteration, the stochastic mini-batch is uniformly sampled with replacement. By the composition of DP with iteration and sampling, the total privacy budget is $(T\frac{m}{n}\epsilon_t, 0)$-DP.
\end{proof}

\section{Proof of Theorem \ref{thm:prob_quant_utility}}\label{app:proof_utilitythm}
% \Utilitythm*
\begin{proof}
    The key to the proof is the boundary of the projection. We consider the two procedures of the projection $\text{Proj}^R_{\calQ_{M,b}}$ is decomposed into two procedures: (a) $\tilde{w}=\mathop{\arg\min}\limits_{x\in\calW}\|x-v\|^2$; (b) $w=\mathop{\arg\min}\limits_{x\in\calQ_r}\|x-\tilde{w}\|^2$.
    % $$\scriptstyle\begin{array}{cc}
    %     \text{(a)} & \tilde{w}=\mathop{\arg\min}\limits_{x\in\calW}\|x-v\|^2 \\
    %     \text{(b)} & w=\mathop{\arg\min}\limits_{x\in\calQ_r}\|x-\tilde{w}\|^2
    % \end{array}$$
    Procedure (b) is a projection of $\tilde{w}$ onto the random quantization set $\calQ_r$. For the projection, we have
    $$\begin{array}{rl}
      \mathop{\mbbE}\limits_{w\in\calQ_r}\left[\tilde{w}-w\right] \leq   & d(\frac{M}{2^b-1})^2\cdot q +d\mathop{\sum}\limits_{i=1}^{2^b-1}(\frac{2M}{2^b-1}i)^2\frac{1-q}{2^b-1}\\
       % \leq & d(\frac{M}{2^b-1})^2 q + d\frac{(2^b-1)2^b(2\cdot2^b-1)}{6}(\frac{2M}{2^b-1})^2\frac{1-q}{2^b-1}\\
       \leq & d M^2\left[\frac{q}{(2^b-1)^2}+\frac{2^{b+1}(2^{b+1}-1)}{3(2^b-1)^2}(1-q)]\right]
    \end{array}$$
     By the triangle inequality, for $u\in\calW$,
    $$\|w-u\|^2\leq\|w-\tilde{w}\|^2+\|\tilde{w}-u\|^2$$
    Let $ e_r=dM^2\left[\frac{q}{(2^b-1)^2}+\frac{2^{b+1}(2^{b+1}-1)}{3(2^b-1)^2}(1-q)]\right]$Combining the above inequalities, we have
    \begin{equation}\label{eq:inequality}
        \|v-u\|^2-\|w-u\|^2\geq- e_r
    \end{equation}

    We next show the excess empirical loss. We assume the loss function is $\rho$-smooth over $\calW$, then for all $w\in\calW$ and $\nabla\in\partial l(w;\cdot)$, we have that $\|\nabla\|\leq \rho$. (Lemma 14.7 in \cite{shalev2014understanding}).

    Since $w_{t+1}$ is the projection of $v_{t}$, and $w^*\in\calW$, we further have 
    $$\scriptstyle\begin{array}{cl}
         & \|w_{t}-w^*\|^2-\|w^{t+1}-w^*\| \\
        \geq & \|w_{t}-w^*\|^2-\|v_{t}-w^*\|^2-e_r\\
        \geq & 2\eta \langle w_t - w^*,\nabla_t\rangle - \eta^2\|\nabla_t\|^2-\eta^2\|G_t\|^2 - e_r
    \end{array}$$
    Taking expectation of both sides, rearranging, and using $\mbbE[\|\nabla_t\|^2]\leq L^2$ and $\mbbE[\|G_t\|^2]= d\sigma^2$ yield
    $$\scriptstyle\begin{array}{cl}
       \langle w_t - w^*,\nabla_t\rangle\leq  & \frac{1}{2\eta}\mbbE[\|w_t-w^*\|^2-\|w_{t+1}-w^*\|^2] \\
         & +\frac{\eta}{2}\rho^2+e_r+\eta\sigma^2 d
    \end{array}$$
    Given that $l$ is convex, we have the bound of $\mbbE\left[\hat{\calL}(\bar{w}_T;\calS)\right]-\mathop{\min}\limits_{w\in\calW}\hat{\calL}(w;\calS)$.
\end{proof}

% \section{Experimental Setup}\label{app:setup}
% The Diagnostic dataset, with 569 30-dimensional instances, was split into $80\%$ training and $20\%$ testing. MNIST contains 70,000 28x28 pixel grayscale images of handwritten digits, split into 60,000 for training and 10,000 for testing.

% \paragraph{Training Details} Two classical ML algorithms - logistic regression (LogReg)~\cite{wright1995logistic}, and support vector machine (SVM)~\cite{hearst1998support} are implemented on the Diagnostic dataset. In particular, we perform linear SVM classifier on the Diagnostic dataset. We implement DP-SGD, DQP-SGD, and RQP-SGD on the training subset. For all experiments on the Diagnostic dataset, we set the mini-batch size as 10. The step size $\eta$ is 1, and the total training iterations is 46. 
% For the LogReg classifier on MNIST, we set the mini-batch size as 64. The step size $\eta$ is 1.0, the total training iteration is 938.
% The clipping norm of the per-sample gradient is $0.45$, the bound of the parameter space is constricted within $[-0.3,0.3]$, and the quantization bit is 4 for quantized training.

% \paragraph{Metrics} \textbf{\textit{Test accuracy:}} the precision of the ML model on the test dataset. \textbf{\textit{Privacy Budget ($\epsilon,\delta$):}} measurement of the privacy constraint of the ML model. 
